# Supplementary material for: Streaming Video Analytics On The Edge With Asynchronous Cloud Support
Source: arXiv:2210.01402 source file (2022-10-04)
Supplement: Supplementary file 1 [file appendix.tex]

\section{Additional Error Diagnostics Results}
\label{sec:appendix-error-analysis}

% \begin{figure*}[h]
%     \centering
%     \includegraphics[width=1.0\columnwidth]{graphs/error_analysis/Error-Diagnostic-Comparison-New.PNG}
%     \caption{Effect of Parameter Choices on Error Breakdown.}
%     % \caption{Cloud detections contribute in decreasing miss rate of \texttt{REACT}. Also, Increase in localization errors correspond with decrease in detection frequencies.}
%     \label{fig:error_analysis_appendix}
% \end{figure*}

\begin{figure}[h]
    \centering
    \includegraphics[width=0.4\columnwidth]{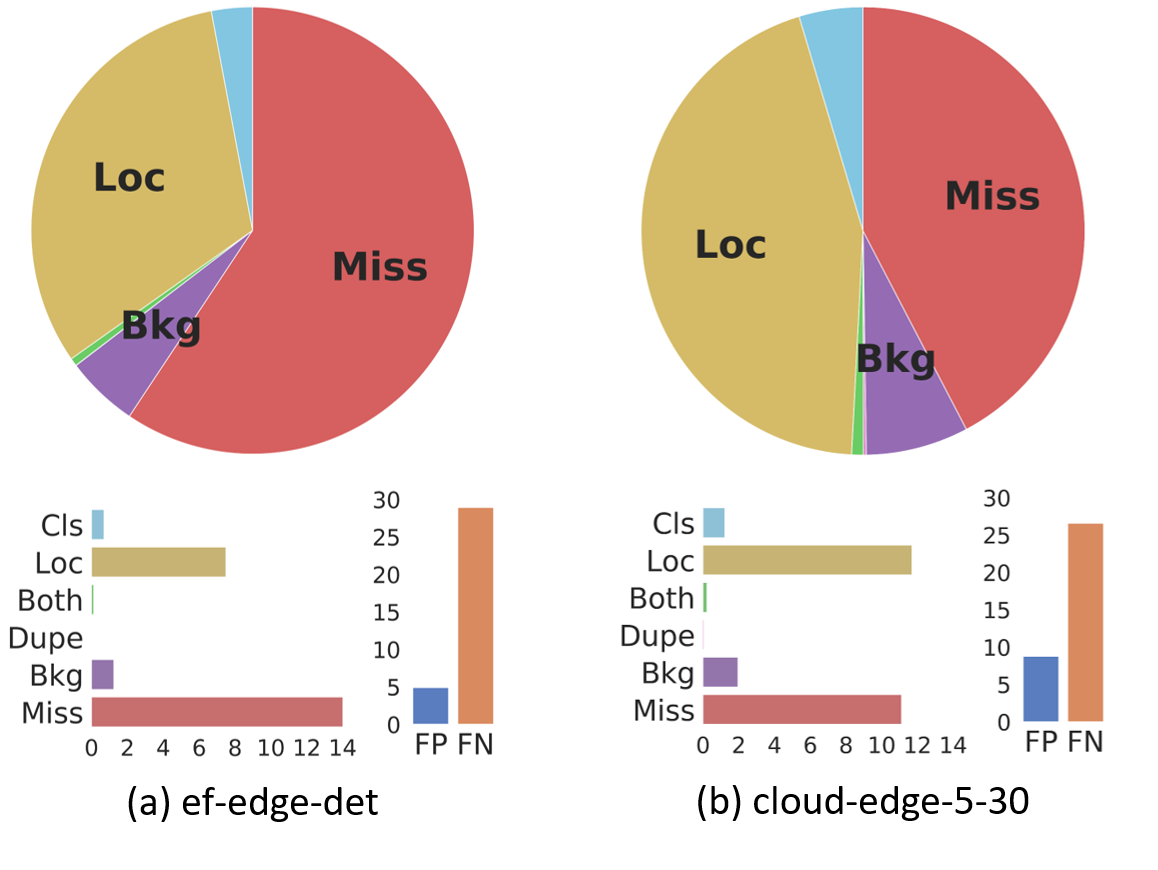}
    \caption{Cloud detections contribute in decreasing miss rate of \pname{} on VisDrone dataset to improve accuracy.}
    % \caption{Cloud detections contribute in decreasing miss rate of \texttt{REACT}. Also, Increase in localization errors correspond with decrease in detection frequencies.}
    \label{fig:error_analysis_appendix_a}
\end{figure}

\begin{figure}[h]
    \centering
    \includegraphics[width=0.4\columnwidth]{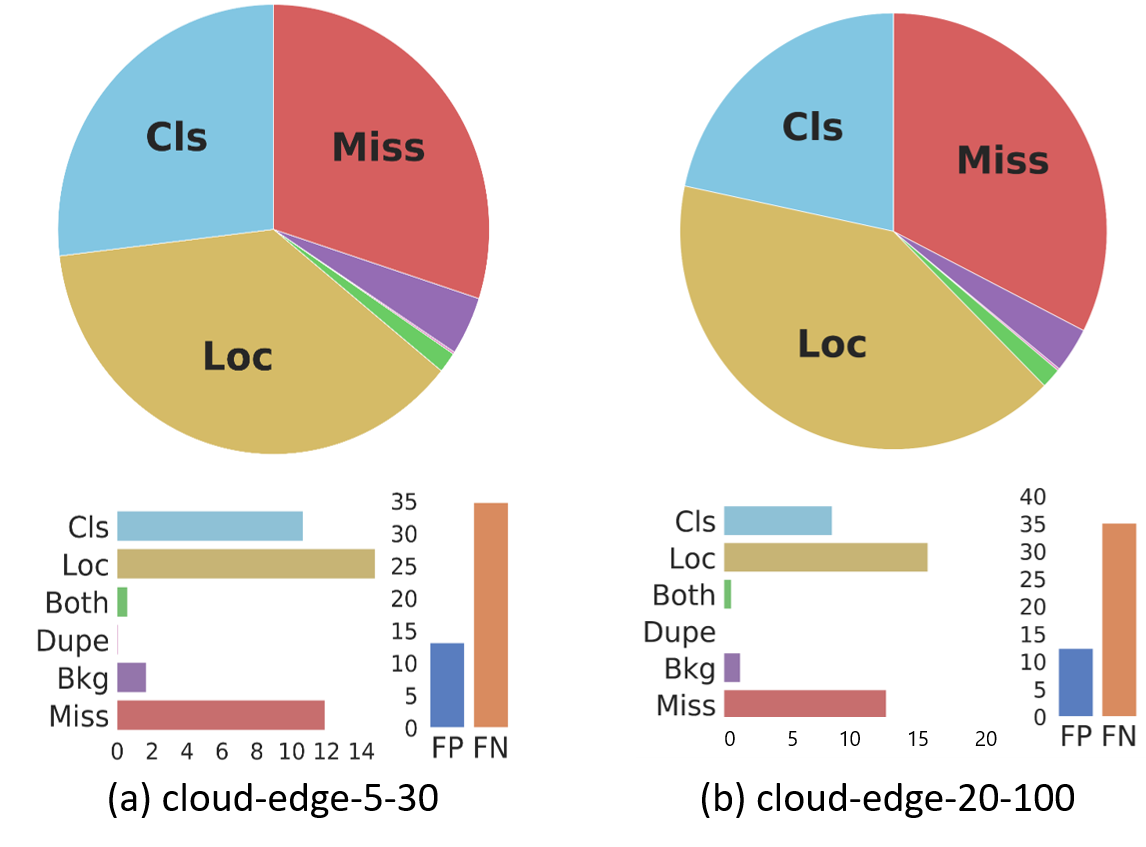}
    \caption{Increase in localization errors correspond with decrease in detection frequencies of \pname{} on D2City Dataset.}
    % \caption{}
    \label{fig:error_analysis_appendix_b}
\end{figure}

We consider two scenarios to demonstrate exactly how cloud detections improve the overall system performance and how parameter choices effect the errors (and mitigation steps). Following Section~\ref{subsec:error-analysis}, we utilize TIDE~\cite{bolya2020tide} to break down the error types for different parameter choices to illustrate the effect of the parameters. TIDE assigns the different error types independently for every detection error (i.e. computes the $\Delta$-mAP, i.e. change in mAP, if an error type was ``fixed'' by an oracle), and thus provides us relative breakdowns that can be compared. This is in contrast with earlier methods (like in COCO Toolkit) which classified all errors progressively (i.e. particular order, and thus summing error breakdown to 1 - mAP score), but that's misleading and is strongly biased toward error types fixed last~\cite{bolya2020tide}.

\textbf{Effect of Cloud Detections}: We analyze the error breakdown between running edge model (tinyYOLO) on every frame and \texttt{REACT} at (5,30) on Visdrone dataset. From Figure~\ref{fig:error_analysis_appendix_a} ((a) and (b)), the ratio of missed detections is substantially lower for \texttt{REACT} contributing to increase in mAP  (See Fig~\ref{fig:cloudpro} (b)) from 10.6 mAP@0.5 to 14.3 mAP@0.5. This indicates is that the cloud models help in detecting objects that edge models are not able to detect (such as small and occluded objects).

\textbf{Effect of System Parameters}: Further, we analyze the results by varying edge and cloud frequency from (5,30) to (20, 100) on D2City dataset. From Figure~\ref{fig:error_analysis_appendix_b} ((a) and (b)), the ratio of localization errors increases as the overall mAP decreases (See Figure~\ref{fig:heat}) from 25 mAP@0.5 to 20.3 mAP@0.5. This indicates that tracker error increases as we reduce the frequencies which could be mitigated by using a more accurate yet more expensive tracker. However, if localization errors are tolerable in the end use-case, for instance in person counting scenarios, then savings in both cloud cost and energy on the edge device can be made.

\section{Additional Scalability Results}
\label{sec:scale}
Figure~\ref{fig:median} shows the $50^{th}$ percentile response time with the increasing number of concurrent edge devices for different GPUs available on Microsoft Azure. 

\begin{figure}[h]
    \centering
     \includegraphics[width=0.4\linewidth]{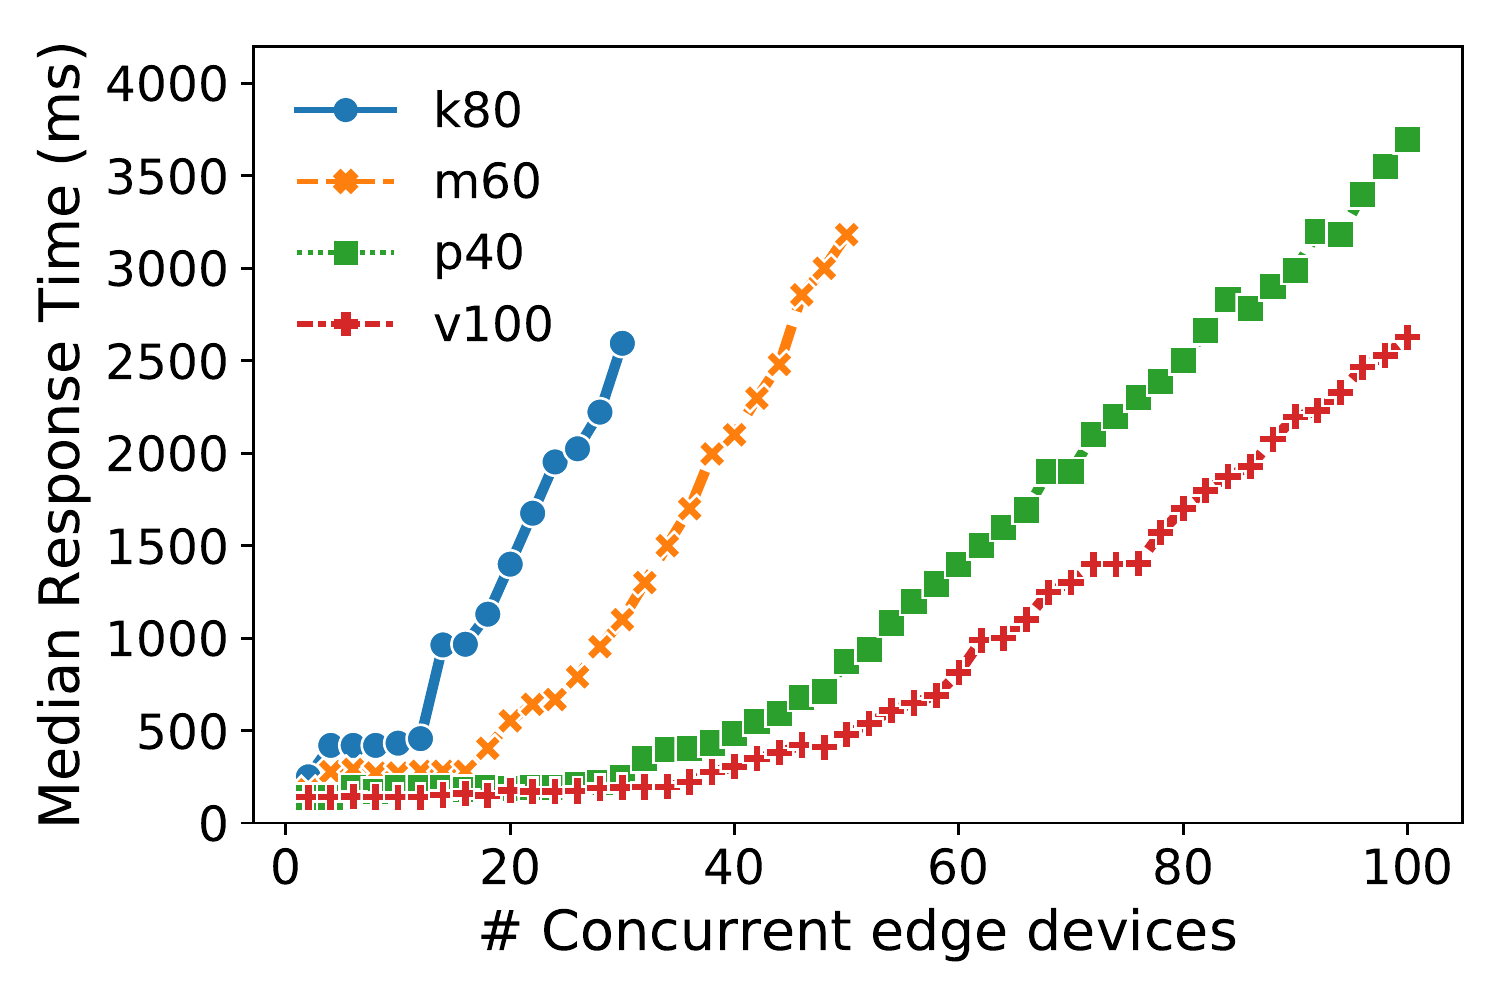}
     \caption{$50^{th}$ percentile response time vs \# concurrent edge devices across GPUs}
     \label{fig:median}
\end{figure}

\section{Visual Results}

\begin{figure*}[h]
    \centering
    \includegraphics[width=0.9\linewidth]{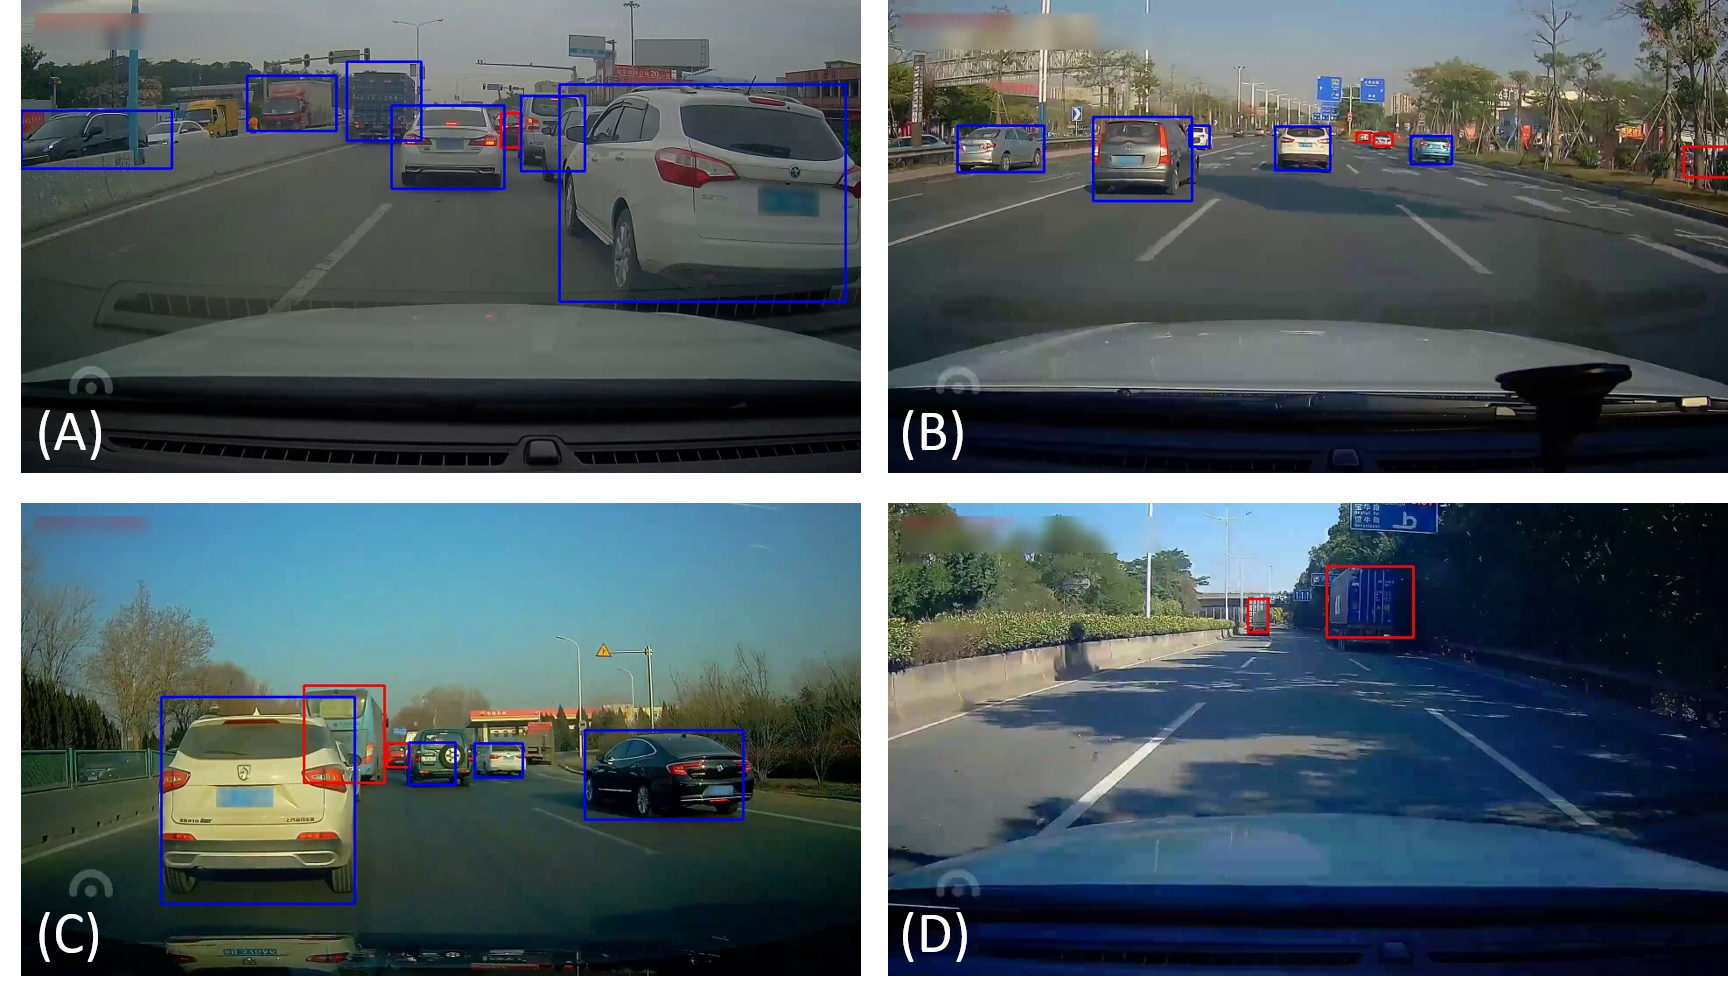}
    \caption{Detections on the D2City dataset. Cloud detections are colored red, whereas Edge detections are colored blue.}
    \label{fig:visual_results_d2city}
\end{figure*}

\begin{figure*}[h]
    \centering
    \includegraphics[width=0.9\linewidth]{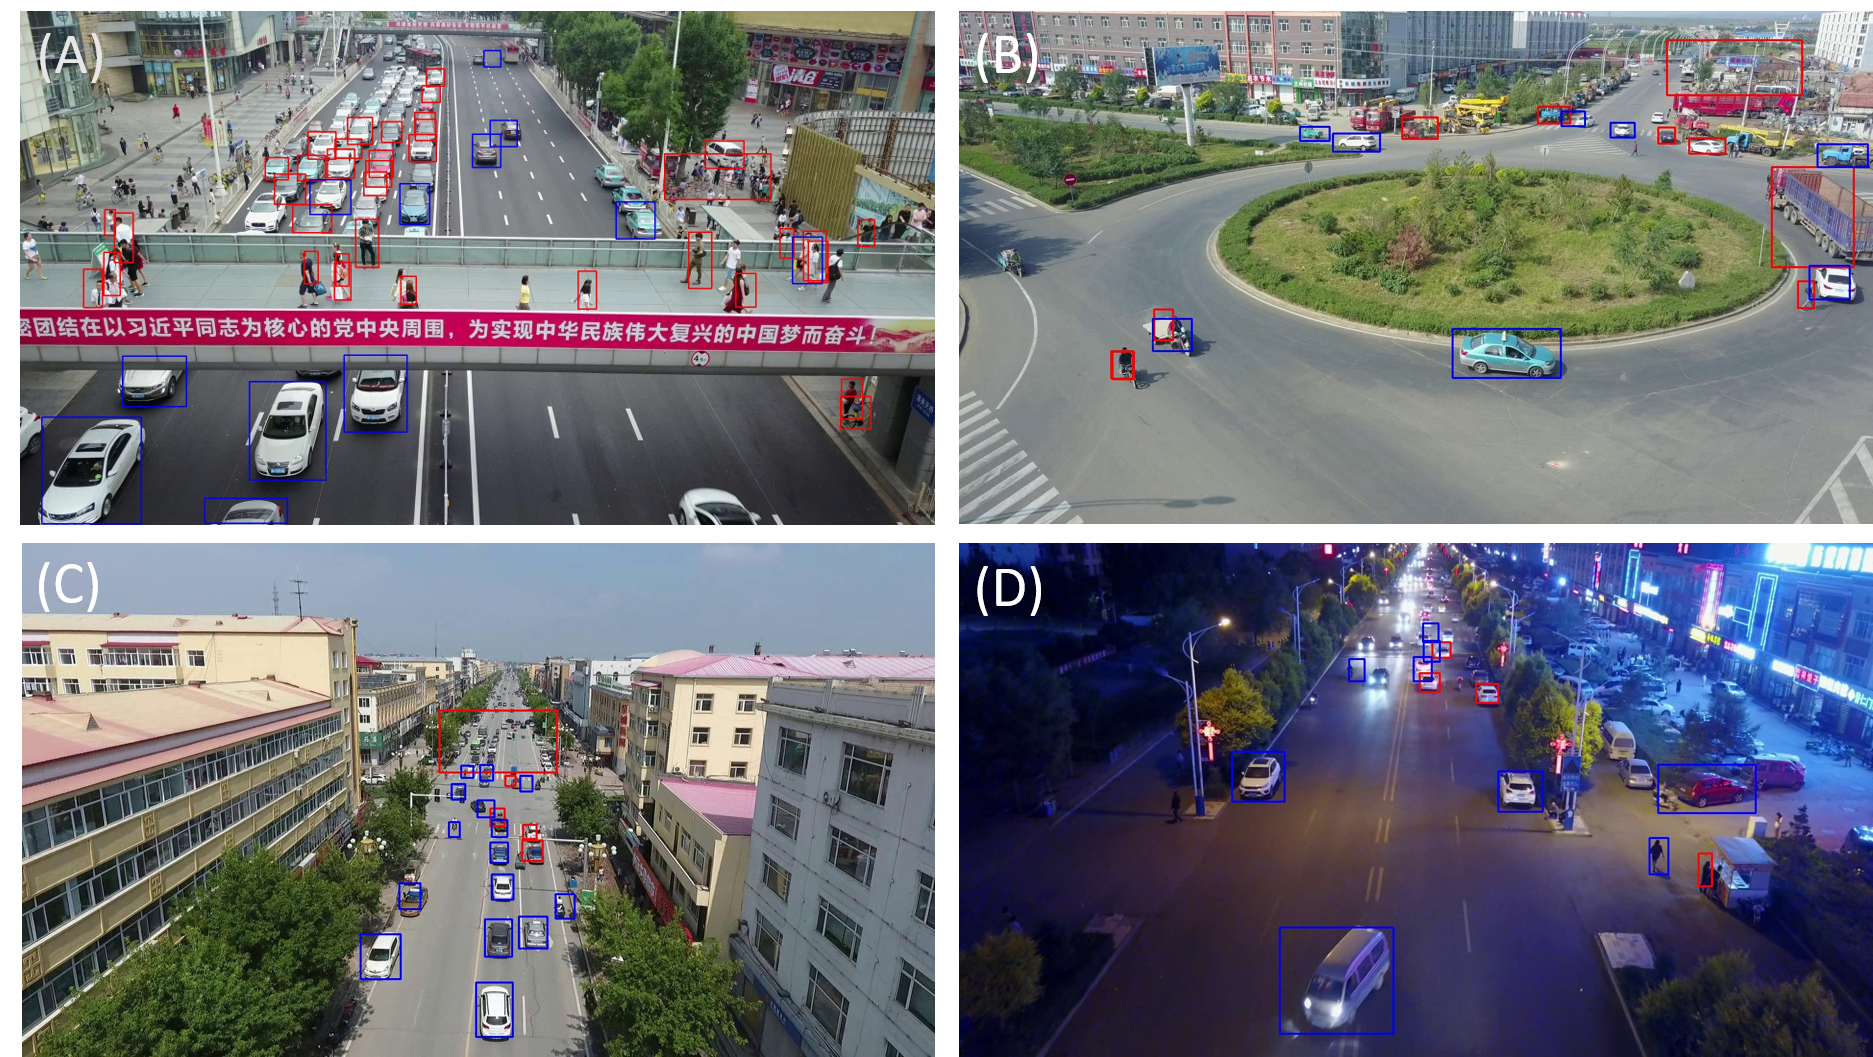}
    \caption{Detections on the Visdrone dataset. Cloud detections are colored red, whereas Edge detections are colored blue.}
    \label{fig:visual_results_visdrone}
\end{figure*}

\label{sec:appendix-visual-results}
% \begin{figure}[h]
%     \centering
%     \includegraphics[width=\columnwidth]{graphs/visual/d2city-visual-results.png}
%     \caption{Detections obtained on the D2City dataset. Cloud detections are colored red, whereas Edge detections are colored blue.}
%     \label{fig:visual_results_d2city}
% \end{figure}

We visualize some frames from various sequences in the D2City dataset using \pname{} with TinyYOLO at the edge and RetinaNet at the cloud with a detection frequency of 5 and 30, respectively. As we can see, \pname{}'s Edge Cloud Fusion Algorithm helps in multiple scenarios. In Fig~\ref{fig:visual_results_d2city} (A), the edge model is able to identify and localize most of the objects, however, cloud model identifies a highly occluded car. While in Fig~\ref{fig:visual_results_d2city} (B), the cloud model is able to identify small objects (such as the \textit{cars} far away) which the edge model could not. The cloud model is able to identify the occluded \textit{bus}, which is close to the camera in Fig~\ref{fig:visual_results_d2city} (C). The edge model performs especially poorly in Fig~\ref{fig:visual_results_d2city} (D), as it's not able to identify any of the \textit{trucks} due to bad lighting conditions, which our cloud model can identify and localize correctly. This is consistent with prior observations that larger models are better at detecting small and occluded objects.

% \begin{figure}[h]
%     \centering
%     \includegraphics[width=\columnwidth]{graphs/visual/visdrone-visual-results.png}
%     \caption{Detections obtained on the Visdrone dataset. Cloud detections are colored red, whereas Edge detections are colored blue.}
%     \label{fig:visual_results_visdrone}
% \end{figure}

Similar patterns emerge in VisDrone dataset, as observed in Fig~\ref{fig:visual_results_visdrone}. Moreover, as we can see in all the sub figures (specially in Fig~\ref{fig:visual_results_visdrone} (A)), the miss rate is significantly reduced by the detection of smaller objects by the cloud model. This is consistent with our observations in Appendix~\ref{sec:appendix-error-analysis} and Fig~\ref{fig:error_analysis_appendix_b}.

% \begin{figure*}
% \centering

% \begin{subfigure}{0.9\textwidth}
%     \centering
%     \includegraphics[width=1\linewidth]{graphs/visual/d2city-visual-results.png}
%     \caption{Detections obtained on the D2City dataset.}
%     \label{fig:visual_results_d2city}
% \end{subfigure}

% \begin{subfigure}{0.9\textwidth}
%     \centering
%     \includegraphics[width=1\linewidth]{graphs/visual/visdrone-visual-results.png}
%     \caption{Detections obtained on the Visdrone dataset.}
%     \label{fig:visual_results_visdrone}
% \end{subfigure}

% \caption{Visual Results on D2City and VisDrone Datasets. Cloud detections are colored red, whereas Edge detections are colored blue.}
% \end{figure*}

% \begin{figure}[h]
%     \centering
%     \includegraphics[width=\columnwidth]{graphs/visual/d2city-visual-results.png}
%     \caption{Detections obtained on the D2City dataset. Cloud detections are colored red, whereas Edge detections are colored blue.}
%     \label{fig:visual_results_d2city}
% \end{figure}

% \begin{figure}[h]
%     \centering
%     \includegraphics[width=\columnwidth]{graphs/visual/visdrone-visual-results.png}
%     \caption{Detections obtained on the Visdrone dataset. Cloud detections are colored red, whereas Edge detections are colored blue.}
%     \label{fig:visual_results_visdrone}
% \end{figure}
%\redX{Add images for different datasets with baseline - Anurag}

%\section{Adaptive Parameter Selection}
